# Supplementary material for: A real neural network state for quantum chemistry
Source: arXiv:2301.03755 source file (2023-01-10)
Supplement: Supplementary file 1 [file appendix.tex]

All calculations and scalability tests were run with FHI-aims on the new generation Sunway supercomputer. For the DFPT calculations of the polarizability tensor, the keyword ``DFPT polar\_reduce\_memory" for finite systems needs to be presented in the control.in files of FHI-aims. In order to perform the distributed storage and adaptive load balancing, the keywords ``use\_local\_index  .true." and ``local\_balancing .true." need to be written into control.in. The key algorithms and optimizations are listed above.

As described in the paper, we use the case of ligand for HIV, RBD and \(H(C_2H4)_nH\) , which can be gotten by ``https://gitee.com/ict-epc/sc22-aims-dfpt/tree/master/testcases" . Test cases are divided into three folders: ``01\_validation", ``02\_performance" and ``03\_scaling", according to the Section Evaluation of the paper. 

Then you can install the code in the following way: (1) tar zxvf FHIaims-opt.tar.gz; (2) cd FHIaims-opt/src (3) make -f Makefile -j 8 scalapack.mpi

After compiling the FHI-aims, there will be a binary file in the FHIaims-opt/bin directory, which is called ``aims.191127.scalapack.mpi.x". Finally, after finishing the compilation, we can go to the directory which contains the control file (control.in) and the geometry file (geometry.in) , and perform the calculation. We can submit the calculation to the queue using : ``bsub -b -m 1 -q queueName -n numProcess -share\_size 4096 -host\_stack 1024 -o output /FHIaims-opt/bin/aims.191127.scalapack.mpi.x"

Relevant hardware details: The new Sunway supercomputer adopts a new generation of domestic high-performance heterogeneous many-core processors (SW39000) in China. Each processor contains 6 core groups (CGs), each CG has one management processing element (MPE), and one computing processing element (CPE) cluster consisting of 64 CPEs. The CPEs are organized as an \(8\times 8\) mesh, with each four sharing a local cluster management unit, which integrates the direct memory access (DMA) engine and the remote memory access (RMA) engine. The MPE is primarily used to handle communication and management tasks, and the CPEs provide most computing performance.  Each core group has a memory controller (MC) that connects to 16GB of DDR4 main memory with a theoretical bandwidth of 51.2GB/s. The main memory can be accessed by the MPE and the CPE cluster in the same CG. Each MPE has a 32KB L1 data/instruction cache and 512KB L2 cache. Each CPE has a 32KB L1 instruction cache and 256KB scratch pad memory (SPM) that can be configured entirely as local data memory controlled by the user, or part of the space can be used as a local data cache under hardware control. The data transmission between the main memory and the SPM is performed by DMA or global load/store instructions, and the data transmission between SPMs of each two CPEs in the same CPE cluster is performed by RMA.

Operating systems and versions: Sunway customized OS with Linux kernel 3.10.0

Compilers and versions: swgcc and swgfortran

Applications and versions: FHI-aims.191127.scalapack.mpi

Libraries and versions: lapack-v3.8.0, scalapack-v2.0.2, SWCH MPI at 20210101
